# Supplementary material for: Spontaneous Symmetry Breaking as a Late-Time Trigger for Interacting Dark Energy
Source: arXiv:2511.14235 source file (2025-11-18)
Supplement: Supplementary file 1 [file supplementary1.pdf]

# Supplementary Material (1) for: *Interacting Dark Energy with Epoch-Dependent Coupling*

Pradosh Keshav MV, Kenath Arun

## Activation Epoch and Growth Diagnostics

We consider two representative activation epochs to probe distinct physical regimes. Matter–radiation equality occurs at $a_{\rm eq} = \Omega_{r0}/\Omega_{m0} \simeq 2.93 \times 10^{-4}$, while matter–DE equality is reached at $a_{\rm DE} = (\Omega_{m0}/\Omega_{\Lambda 0})^{1/3} \simeq 0.772$. The benchmark choice $a_c = 0.01$ therefore corresponds to activation well inside the matter-dominated era, potentially influencing structure formation, whereas $a_c = 0.71$ represents a late activation near the onset of DE domination, affecting only the most recent evolution. To track the system through both symmetric ($\mu^2_{\rm eff} > 0$) and broken ($\mu^2_{\rm eff} < 0$) phases, we computed the numerically realized transition epoch $a_c^{\rm num}$, the fractional displacement from the asymptotic minimum $|\delta|/v_0 \equiv |v(a) - v_0|/v_0$, and the adiabaticity ratio $|m^2_\phi|/H^2$ with $m^2_\phi(a) = 2\lambda\,[3v(a)^2 - v_0^2]$. These estimates quantify when the adiabatic-tracking and small-shift approximations are valid: Figure 1 show that in the symmetric phase ($a < a_c$), $\mu^2_{\rm eff}(a) > 0$ pins the minimum at $v(a) = 0$, with $\beta(a) = 0$ indicating negligible CDM–DE interaction. At $a \simeq a_c$, the sign flip in $\mu^2_{\rm eff}$ drives the scalar to acquire a vacuum value, triggering a sharp but continuous rise in $\beta(a)$ toward its late-time saturation. This activation era thus plays the role of an order parameter: both $v(a)$ and $\beta(a)$ rise from zero to $\mathcal{O}(1)$ after the transition. An early activation at $a_c = 0.01$ leaves $\beta(a)$ nearly constant during structure formation, whereas a late activation at $a_c \simeq 0.7$ delays the onset until DE domination.

Table 1 quantifies these trends. In both early and late cases, the displacement peaks at $\max|\delta|/v_0 \simeq 0.85$ near the transition, briefly challenging the small-shift approximation, but the subsequent evolution is strongly adiabatic: $\min(|m^2_\phi|/H^2) \gg 1$ for $a > a_c$, and a rapid relaxation to $v(a)$. Present-day displacements remain under perturbative control, being negligible for $a_c = 0.01$ and modest ($\sim 0.20$) for $a_c \simeq 0.7$. The late-time coupling is close to saturation in both cases, with $\beta(a = 1)/\beta_0 \simeq 1.0$ (early) and $\simeq 0.8$ (late), implying an effective fifth force $\sim \beta^2 G$ at $z = 0$, comparable to gravity for $\beta_0 = \mathcal{O}(1)$. However, microphysical implications differ substantially in all the above cases. In the early-activation case, small values of the density-induced parameter $\xi$ and Yukawa coupling $g$ suffice to trigger SSB during matter domination, whereas delaying activation to $a_c \simeq 0.7$ requires larger couplings, consistent with postponing symmetry breaking until dark-energy domination. Overall, these diagnostics infer that the rise of $\beta(a)$ is a genuine order-parameter effect of SSB-induced coupling with a distinct observational signature on late-time growth.

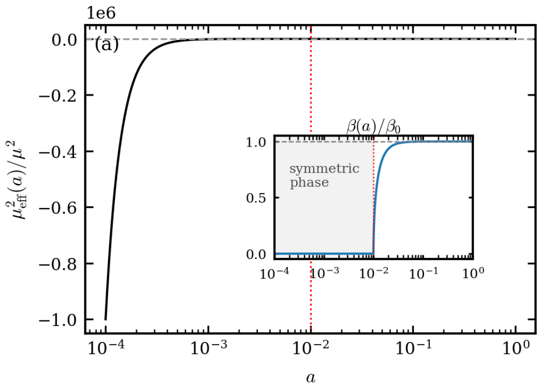


(a) $\mu^2_{\rm eff}(a)/\mu^2$ with inset showing $v(a)/v_0$ and $\beta(a)/\beta_0$ for $a_c = 0.01$.

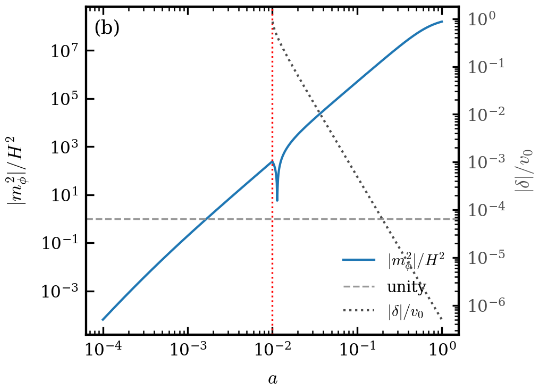


(b) Adiabaticity ratio $|m^2_\phi|/H^2$ (solid) and fractional displacement $|\delta|/v_0$ (dotted) for $a_c = 0.01$.

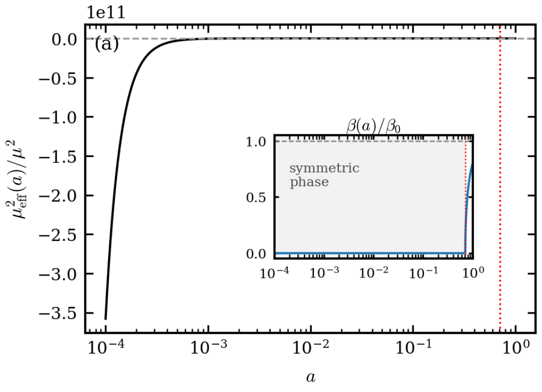


(c) $\mu^2_{\rm eff}(a)/\mu^2$ with inset showing $v(a)/v_0$ and $\beta(a)/\beta_0$ for $a_c = 0.71$.

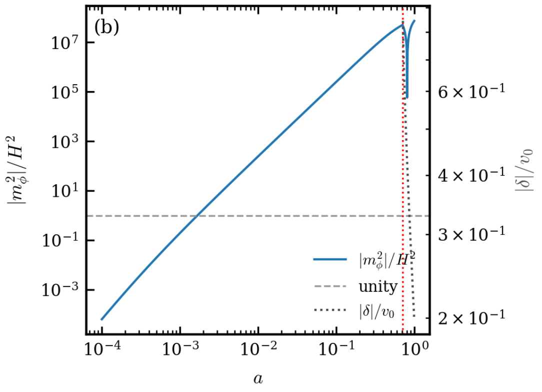


(d) Adiabaticity ratio $|m^2_\phi|/H^2$ (solid) and fractional displacement $|\delta|/v_0$ (dotted) for $a_c = 0.71$.

Figure 1: Left panels: effective mass-squared ratio $\mu^2_{\rm eff}(a)/\mu^2$ (solid) with transition point $a_c$ marked (vertical dashed). Insets display the vacuum expectation value $v(a)/v_0$ (solid) and normalized coupling $\beta(a)/\beta_0$ (dashed). Right panels: adiabaticity ratio $|m^2_\phi|/H^2$ (solid) compared to unity threshold (horizontal dashed), together with fractional displacement $|\delta|/v_0$ (dotted). For $a_c = 0.01$, the coupling activates early and remains constant through most of structure formation; for $a_c = 0.71$, the activation is late, leaving early-time dynamics ΛCDM-like while allowing late-time modification of $G_{\rm eff}$. In both cases, $\min(|m^2_\phi|/H^2) \gg 1$ after the transition, ensuring adiabatic tracking.

Table 1: Diagnostics for two benchmark activation epochs. Columns report fiducial microphysics, derived effective parameters $(\mu^2, \xi, g)$, and cosmological checks. Both scenarios are strongly adiabatic, with $\beta(a)$ exhibiting the expected SSB order-parameter behavior. However, they differ in the timing of activation: early activation at $a_c = 0.01$ results in a constant coupling throughout structure formation, while late activation at $a_c = 0.71$ mimics the early growth of a ΛCDM model and only modifies the DE era.

| Quantity | $a_c^{\rm target} = 0.01$ | $a_c^{\rm target} = 0.7$ | SSB analogy | Comments |
|---|---|---|---|---|
| $v_0/M_{\rm Pl}$ | $\sim 10^{-5}$ | $\sim 10^{-5}$ | Bare VEV scale | Fixes late-time $\beta$ amplitude |
| $\lambda$ | $\sim 10^{-1}$ | $\sim 10^{-1}$ | Quartic self-coupling | Steepness of scalar potential |
| $\mu^2$ | $3.77 \times 10^{-28}$ | $3.77 \times 10^{-28}$ | Tachyonic mass$^2$ | Onset of instability / SSB trigger |
| $\xi$ | $1.66 \times 10^{-7}$ | $5.94 \times 10^{-2}$ | Density–induced mass shift | Controls location of $a_c$ |
| $g$ | $9.87 \times 10^{-33}$ | $3.53 \times 10^{-27}$ | CDM–scalar Yukawa coupling | Strength of scalar–DM force |
| $a_c^{\rm num}$ | 0.010 | 0.716 | Critical point of SSB | Activation epoch in cosmic history |
| $\max\lvert\delta\rvert/v_0$ | $8.69 \times 10^{-1}$ | $8.44 \times 10^{-1}$ | Maximal excursion | Size of non-adiabatic transient |
| $\lvert\delta\rvert/v_0$ $(a = 1)$ | $5.0 \times 10^{-7}$ | $1.99 \times 10^{-1}$ | Residual displacement | Validity of perturbative expansion today |
| $\min(\lvert m_\phi^2\rvert/H^2)_{a>0.1}$ | $5.11 \times 10^5$ | $5.84 \times 10^4$ | Adiabaticity check | Ensures tracking of $v(a)$ after $a_c$ |
| $\beta(a = 1)/\beta_0$ | $\approx 1.00$ | $\approx 0.80$ | Order parameter | Effective coupling strength today |
