# Supplementary material for: Spontaneous Symmetry Breaking as a Late-Time Trigger for Interacting Dark Energy
Source: arXiv:2511.14235 source file (2025-11-18)
Supplement: Supplementary file 2 [file supplementary2.pdf]

# Supplementary Material (2) for: *Interacting Dark Energy with Epoch-Dependent Coupling*

Pradosh Keshav MV, Kenath Arun

## Diagnostic of the Interaction Strength $\Gamma_Q$

The impact of the interaction is expected to be negligible before the activation epoch, so freezing $H(a)$ to its $\Lambda$CDM form allows us to cleanly isolate the perturbation-level effects of $\beta(a)$ on structure growth. Running a fully self-consistent background+perturbation integration across the entire posterior would be considerably more computationally expensive, as it requires solving stiff, coupled dynamical equations for each MCMC draw while simultaneously propagating CMB distance priors.

For completeness we state the interaction current used in the diagnostics. In our convention

$$Q(a) \; = \; \frac{\beta(a)}{M_{\rm Pl}}\,\rho_m(a)\,\dot{\phi}(a),$$

so that the fractional interaction diagnostic reduces to

$$\Gamma_Q(a) \equiv \frac{|Q|}{3H\rho_m} \; = \; \frac{|\beta(a)|}{3}\,\frac{|\dot{\phi}|}{M_{\rm Pl}H}.$$

Under the conservative adiabatic scaling used for the fast scan, $\dot{\phi}/M_{\rm Pl} \sim H$, we therefore obtain the approximate relation

$$\Gamma_Q(a) \simeq \frac{|\beta(a)|}{3},$$

which enables rapid posterior exploration without full ODE integration. The adiabatic approximation and its range of validity are explicitly checked by exact re-integrations for the highest-impact draws.

We drew $N = 400$ samples from both the Planck-included and no-Planck flattened chains and evaluated $\Gamma_Q(z)$ on the interval $0 \leq z \leq 3$. For the Planck-included posterior we find median($\max_z \Gamma_Q$) $\simeq 2.80 \times 10^{-2}$ with 16–84% range $[8.42 \times 10^{-3}, 5.85 \times 10^{-2}]$ and 2.5–97.5% range $[1.48 \times 10^{-3}, 8.52 \times 10^{-2}]$. Approximately 99.3% of drawn samples satisfy $\max_z \Gamma_Q < 10^{-1}$, while 17.2% and 2.0% of samples satisfy $\max_z \Gamma_Q < 10^{-2}$ and $\max_z \Gamma_Q < 10^{-3}$, respectively. By contrast, for the posterior obtained without the Planck compressed prior the interaction is substantially larger: median($\max_z \Gamma_Q$) $\simeq 1.70 \times 10^{-1}$ with 16–84% range $[1.08 \times 10^{-1}, 2.18 \times 10^{-1}]$ and 2.5–97.5% range $[1.82 \times 10^{-2}, 2.59 \times 10^{-1}]$. In this case

only 14.0% of draws satisfy $\max_z \Gamma_Q < 10^{-1}$, with 0.5% and 0.0% falling below the $10^{-2}$ and $10^{-3}$ thresholds, respectively. The fast-scan bands are shown in Fig. 1 (Planck-included and no-Planck overplotted), and summary statistics are given in Table 1.

For the Planck-included top samples, the exact integrations are consistent with the adiabatic forecast, and the change in total $\chi^2$ when replacing the frozen background by the exact $H(a)$ is small, with $\Delta\chi^2 \lesssim 0.5$ for all tested draws. Using the adiabatic diagnostic described above, we computed the cumulative fractional change in the Hubble rate,

$$\frac{\Delta H}{H}(z) \simeq \frac{1}{2} \frac{\int_{a(z)}^{1} \beta(a')\, \rho_m(a')\, \frac{da'}{a'}}{\rho_{\rm tot}(a)},$$

for $N_{\rm draw} = 400$ random posterior samples from each chain. For the Planck-included posterior, we find

$$\begin{aligned} \mathrm{median}\Big(\max_z \Delta H/H\Big) &= 8.073 \times 10^{-3}, \\ 16\text{–}84\% &= [2.789 \times 10^{-3},\, 1.862 \times 10^{-2}], \\ 2.5\text{–}97.5\% &= [4.042 \times 10^{-4},\, 2.994 \times 10^{-2}]. \end{aligned}$$

For the posterior obtained without the Planck compressed prior the interaction induces substantially larger background shifts:

$$\begin{aligned} \mathrm{median}\Big(\max_z \Delta H/H\Big) &= 4.853 \times 10^{-2}, \\ 16\text{–}84\% &= [3.290 \times 10^{-2},\, 6.417 \times 10^{-2}], \\ 2.5\text{–}97.5\% &= [9.376 \times 10^{-3},\, 8.329 \times 10^{-2}]. \end{aligned}$$

These numbers imply that for the Planck-included ensemble, the integrated background correction is typically below the percent level (median $\approx$ 0.8%), while for the no-Planck ensemble, cumulative corrections are several percent and cannot be neglected. Accordingly, we carried out exact ODE re-integrations (coupled Klein–Gordon + CDM continuity + Friedmann) for the highest-impact Planck-included draws and confirm that the change in full likelihood is small (see Table 1 and Fig. 2). We therefore present the Planck-included results in the main text using the frozen background, which is validated by these diagnostics. For completeness, exploratory constraints from the no-Planck chains are reported in Tables 2 and 3, but these should be interpreted only as dataset-sensitivity tests since a self-consistent background evolution is required for that ensemble. All diagnostic data files (fast-scan arrays, exact re-check tables, and figures) can be provided upon request.

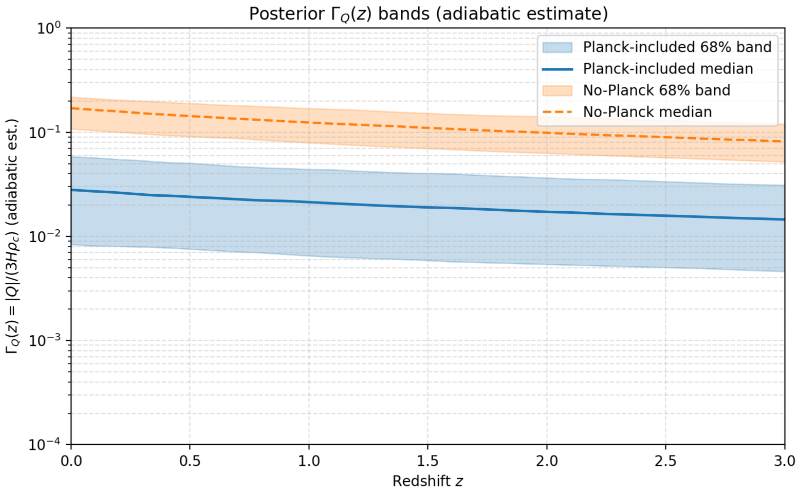


Figure 1: Posterior bands for the adiabatic estimate of the interaction diagnostic $\Gamma_Q(z) = |Q|/(3H\rho_m) \simeq \beta(a)/3$. Shaded regions show the 68% credible band and lines the posterior median, computed from $N = 400$ random draws of the flattened chains. The Planck-included chain (solid) is pushed toward a smaller $\Gamma_Q$ compared with the no-Planck chain (dashed), which exhibits substantially larger interaction strengths for a large fraction of the posterior.

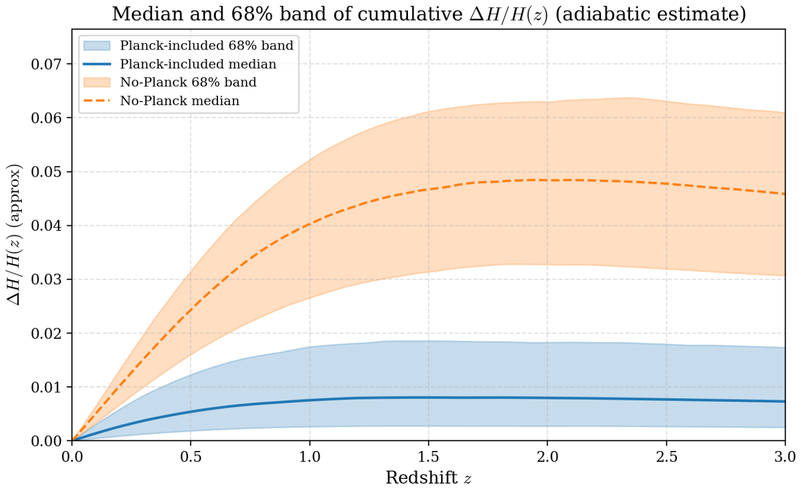


Figure 2: Cumulative fractional change in the Hubble expansion, $\Delta H/H(z)$, estimated from the adiabatic diagnostic $\Delta H/H \simeq \frac{1}{2}\Delta\rho_m/\rho_{\rm tot}$ using $N = 400$ posterior draws. Solid lines show the posterior median and shaded regions the 68% credible band. The Planck-included posterior (blue) yields median $\max_z \Delta H/H \simeq 8 \times 10^{-3}$ with a 97.5th percentile $\simeq 3 \times 10^{-2}$, indicating that background corrections remain at the sub-percent to few-percent level. In contrast, the no-Planck posterior (orange, dashed) exhibits substantially larger cumulative shifts, with typical $\Delta H/H$ at the several-percent level. These diagnostics demonstrate that freezing $H(a)$ to the $\Lambda$CDM background is a safe approximation for the Planck-constrained ensemble, while the no-Planck results require a self-consistent background treatment.

| Statistic | Planck-included ($N_{draw} = 400$) | No-Planck ($N_{draw} = 400$) |
|---|---|---|
| Median ($\max \Gamma_Q$) | $2.797 \times 10^{-2}$ | $1.704 \times 10^{-1}$ |
| 16 / 84 percentile | $8.415 \times 10^{-3} / 5.852 \times 10^{-2}$ | $1.078 \times 10^{-1} / 2.183 \times 10^{-1}$ |
| 2.5 / 97.5 percentile | $1.475 \times 10^{-3} / 8.520 \times 10^{-2}$ | $1.816 \times 10^{-2} / 2.586 \times 10^{-1}$ |
| Fraction ($\max \Gamma < 10^{-1}$) | 0.993 | 0.140 |
| Fraction ($\max \Gamma < 10^{-2}$) | 0.172 | 0.005 |
| Fraction ($\max \Gamma < 10^{-3}$) | 0.020 | 0.000 |

Table 1: Comparison of Planck-included vs. No-Planck results over $N_{\text{draw}} = 400$ samples for the maximum $\Gamma_Q$.

Table 2: Posterior constraints for the epoch-dependent coupling model ($n = 1$) from RSD+BAO+CC+Pantheon+SH0ES without Planck compressed priors. Quoted values are posterior mean $\pm 1\sigma$; 68% and 95% credible intervals are shown where useful. These results are exploratory since the frozen-background approximation is less reliable without Planck constraints (see Supplementary Fig. 2).

| Parameter | Mean $\pm 1\sigma$ | 68% C.L. | 95% C.L. |
|---|---|---|---|
| $\Omega_m$ | $0.1993 \pm 0.0063$ | $0.1992^{+0.0063}_{-0.0063}$ | $0.1992^{+0.0121}_{-0.0123}$ |
| $H_0$ ($\mathrm{km\,s^{-1}Mpc^{-1}}$) | $76.44 \pm 0.16$ | $76.43^{+0.16}_{-0.16}$ | $76.43^{+0.32}_{-0.32}$ |
| $\sigma_{8,0}$ | $0.77 \pm 0.05$ | $0.77^{+0.05}_{-0.05}$ | $0.77^{+0.09}_{-0.10}$ |
| $\beta_0$ | $0.77 \pm 0.31$ | $0.77^{+0.31}_{-0.31}$ | $0.77^{+0.60}_{-0.67}$ |
| $a_c$ | $0.568 \pm 0.278$ | $0.597^{+0.281}_{-0.359}$ | $0.597^{+0.384}_{-0.553}$ |
| $\Omega_b h^2$ | $0.0225 \pm 0.0020$ | $0.0225^{+0.0024}_{-0.0024}$ | $0.0225^{+0.0033}_{-0.0034}$ |

Table 3: Planck compressed-prior diagnostic and $\chi^2$ breakdown evaluated at the no-Planck posterior mean. For Planck uncertainties we use $\sigma_R = 4.6 \times 10^{-3}$, $\sigma_{\ell_A} = 0.09$, and $\sigma_{\Omega_b h^2} = 1.5 \times 10^{-4}$ (Planck 2018 compression). The $\Delta/\sigma$ column shows the offset in Planck sigma units. These large shifts highlight why the no-Planck runs should be treated as exploratory.

| Quantity | Planck value | Posterior mean (no-Planck fit) | $\Delta/\sigma_{\text{Planck}}$ |
|---|---|---|---|
| $R$ | 1.7502 | 1.7933 | $\approx 9.4\sigma$ |
| $\ell_A$ | 301.471 | 282.87 | (see note) |
| $\Omega_b h^2$ | 0.02236 | 0.02330 | $\approx 6.3\sigma$ |
| **$\chi^2$ breakdown (at no-Planck posterior mean)** | | | |
| Dataset | $N$ | $\chi^2$ | $\chi^2/N$ |
| SNe (Pantheon+SH0ES) | 1701 | 1792 | 1.05 |
| RSD | ∼20 | 31.8 | 1.6 |
| BAO | 26 | 56.5 | 2.1 |
| CC | 31 | 22.4 | 0.7 |
| Planck compressed priors | 3 | $5.34 \times 10^4$ | – |
| Total | 1781 | $5.50 \times 10^4$ | – |

**Note:** The very large $\ell_A$ offset requires a consistency check of the acoustic-scale convention used for the Planck compression (e.g. whether $r_s$ evaluated at the drag epoch $z_d$ or at last scattering $z_*$ is used). If conventions match, the numbers indicate a genuine high-significance geometric tension between the low-$z$ best-fit region and Planck.
